# Supplementary material for: Parameterized Complexity of Locally Minimal Defensive Alliances
Source: arXiv:2105.10742 source file (2023-03-03)
Supplement: Supplementary file 1 [file appendix.tex]

\section{An Illustration of the Algorithm in Section \ref{tree-algo}}
Consider the tree shown in Figure \ref{tree}.
\begin{figure}[ht]
     \centering
    \[\begin{tikzpicture}[scale=0.6]
	%% Notice in the first vertex is named (v) for the sake of a later edge,
	%% and it also has a label to its left that is the math-mode $v$. 
	\vertex (x1) at (0,0) [label=above:$x_1$] {};  
	\vertex (x2) at (-1,-1) [label=left:$x_2$] {};
	\vertex (x3) at (1,-1) [label=right:$x_3$] {};
	\vertex (x4) at (0,-2) [label=below:$x_4$] {};
	\vertex (x5) at (2,-2) [label=right:$x_5$] {};
	\vertex (x6) at (3, -3) [label=right:$x_6$] {};
	\path
	   % Note that the word "path" here isn't used in the graph-theory sense; the \path command
	   % is always used prior to the list of edges; here, coincidentally, they do form an actual path.
		(x1) edge (x2)
		(x1) edge (x3)
		(x3) edge (x4)
		(x3) edge (x5)
		(x5) edge (x6)
		;   % This semicolon ends the \path command.
\end{tikzpicture}\]
\caption{The largest locally minimal strong defensive alliances of $T$ are $\{x_{1},x_{3},x_{4}\}$ and $\{x_{1},x_{3},x_{5}\}$}
     \label{tree}
 \end{figure}
For a leaf node $x\in \{x_2,x_4,x_6\}$, we have  $A_x(0)=0$, $A_x(m_{g}^{p})=A_x(o_{g}^{p})=A_x(o_{g}^{\bar{p}})=A_x(m_{g}^{\bar{p}})=A_x(o_{b}^{p})=-\infty$ and \\ $A_x(m_{b}^{p})=1$.
 For non-leaf node
$x_5$, we have $ A_{x_5}(0)= \max\Big\{A_{x_6}(0), A_{x_6}(m_{g}^{\bar{p}}), A_{x_6} (o_{g}^{\bar{p}})\Big\}=\max\{0, -\infty, -\infty\}=0$. Since $d=1$, we have $A_{x_{5}}(m^{p}_{g})= -\infty$ and $\lceil\frac{d+1}{2}\rceil-1=0$. Therefore
\begin{equation*}
A_{x_{5}}(m_{g}^{\bar{p}}) = 1 + \max\{A_{x_{6}}(m^{p}_{g}),A_{x_{6}}(m^{p}_{b})\}=1 + \max\{-\infty,1\} =2 
\end{equation*}
and
\begin{equation*}
A_{x_{5}}(o_{g}^{p})  = A_{x_{5}}(o_{g}^{\bar{p}})  = 1 + A_{x_{5}}(m^{p}_{g}) = 1+ (-\infty) = -\infty.
\end{equation*}
Next, we consider the states $o^{p}_{b}$ and $m^{p}_{b}$. We have 
$A_{x_{5}}(o_{b}^{p}) = 1 + A_{x_{5}}(o^{p}_{g}) = 1 + (-\infty) = -\infty$
and $A_{x_{5}}(m_{b}^{p}) = 1 $.
For non-leaf node $x_3$, we have $d=2$; 
\begin{equation*}
\begin{split}
A_{x_3}(0) &= \max\Big\{A_{x_4}(0), A_{x_4}(m^{\bar{p}}_{g}), A_{x_4} (o^{\bar{p}}_{g}), A_{x_5}(0), A_{x_5}(m^{\bar{p}}_{g}), A_{x_5} (o^{\bar{p}}_{g})\Big\} \\
&= \max\{0,-\infty,-\infty,0,2,-\infty \}=2
\end{split}    
\end{equation*}
 and the associated locally minimal defensive
 alliance is $\{x_5,x_6\}$. For the state  $m^p_g$, we have
 \begin{equation*} 
\begin{split}
 A_{x_3}(m^{p}_{g})& =1+\max\limits_{x\in \mathcal{C}_1}\{\max\Big\{ A_x(1_{og}), A_x (1_{ob})\Big\} \}\\
 &= 1+\max\Big\{ A_{x_4}(m^{p}_{g}), A_{x_4}(m^{p}_{b}),A_{x_5}(m^{p}_{g}), A_{x_5}(m^{p}_{b})\Big\}\\
 &=1+ \max\{-\infty,1,-\infty, 1\}=2.
\end{split}
\end{equation*}
For the state $m^{\bar{p}}_g$, we have
\begin{equation*} 
\begin{split}
A_{x_3}(m^{\bar{p}}_{g})& =1+\max \Big\{ \max \Big\{ A_{x_{4}}(m^{p}_{g}), A_{x_{4}} (m^{p}_{b})\Big\} + \max\Big\{ A_{x_{5}}(m^{p}_{g}), A_{x_{5}}(m^{p}_{b}), A_{x_{5}}(o^{p}_{g}), A_{x_{5}}(o^{p}_{b}) \Big\}, \\
 &\max \Big\{ A_{x_{5}}(m^{p}_{g}), A_{x_{5}} (m^{p}_{b})\Big\} + \max\Big\{ A_{x_{4}}(m^{p}_{g}), A_{x_{4}}(m^{p}_{b}), A_{x_{4}}(o^{p}_{g}), A_{x_{4}}(o^{p}_{b}) \Big\} \Big\}\\
 &=1+ \max\{2,2\}=3, 
\end{split}
\end{equation*}
and the associated locally minimal defensive
 alliances are $\{x_3,x_4,x_5\}$ and $\{x_3,x_5,x_6\}$. Next, we get
 \begin{equation*} 
\begin{split}
    A_{x_{3}}(o^{p}_{g}) &= 1 + \max \Big\{ A_{x_{4}}(m^{p}_{g}) + \max \Big\{ A_{x_{5}}(m^{p}_{g}),A_{x_{5}}(o^{p}_{g}), \\
    & A_{x_{5}}(m^{p}_{g}) + \max \Big\{ A_{x_{4}}(m^{p}_{g}),A_{x_{4}}(o^{p}_{g})\Big\} \Big\}\\
    &= 1 + \max\{-\infty,-\infty\}=-\infty
\end{split}
\end{equation*}
Similarly, since $A_{x_{4}}(m^{p}_{g}) = A_{x_{5}}(m^{p}_{g}) = -\infty $, we get $A_{x_{3}}(o^{\bar{p}}_{g}) = -\infty$. As $A_{x_{4}}(o^{p}_{g}) = A_{x_{5}}(o^{p}_{g}) = -\infty $,  we get $A_{x_{3}}(o^{p}_{b})=1+(-\infty)=-\infty$. As 
$A_{x_{4}}(o^{p}_{g})= A_{x_{4}}(o^{p}_{b})= A_{x_{5}}(o^{p}_{g})= A_{x_{5}}(o^{p}_{b})= -\infty$, we get $A_{x_{3}}(m^{p}_{b})= 1 + (-\infty) = -\infty$.
Finally, for the root 
node $x_1$, we have $d=2$ and  
\begin{equation*} 
\begin{split}
A_{x_1}(0) &= \max\Big\{A_{x_2}(0), A_{x_2}(m_{g}^{\bar{p}}), A_{x_2} (o_{g}^{\bar{p}}), A_{x_3}(0), A_{x_3}(m_{g}^{\bar{p}}), A_{x_3} (o_{g}^{\bar{p}})\Big\}\\
&= \max\{0,-\infty,-\infty,2,3,-\infty\}=3.
\end{split}
\end{equation*}
As $A_{x_{2}}(m^{p}_{g}) = A_{x_{3}}(m^{p}_{g}) = -\infty $, 
we get $A_{x_{1}}(o^{\bar{p}}_{g})=-\infty$. Next
\begin{equation*} 
\begin{split}
A_{x_{1}}(m^{\bar{p}}_{g}) &= 1 + \max \Big \{ \max\{ A_{x_{2}}(m^{p}_{g}),A_{x_{2}}(m^{p}_{b})\}, \max\{A_{x_{3}}(m^{p}_{g}),A_{x_{3}}(m^{p}_{b})\}  \Big\}\\
&= 1+2=3.
\end{split}
\end{equation*}
The associated connected locally minimal strong defensive alliances are $\{x_{1},x_{3},x_{4}\}$ and $\{x_{1},x_{3},x_{5}\}$.
Therefore, the size of the largest locally minimal strong defensive alliance is 
$\max\{A_{x_1}(0),A_{x_1}(m^{\bar{p}}_{g}),A_{x_1}(o^{\bar{p}}_{g})\}=3$.
